# Supplementary material for: Efficient construction of generalized master equation memory kernels for multi-state systems from nonadiabatic quantum-classical dynamics
Source: arXiv:1903.09608 ancillary file (2019-06-26)
Supplement: Supplementary file 1 [file Supplement.pdf]

**Efficient construction of generalized master equation memory kernels for multi-state systems from nonadiabatic quantum-classical dynamics**

William C. Pfalzgraff, Andrés Montoya-Castillo, Aaron Kelly, Thomas E. Markland

## Supporting Information

## 1. Memory kernel matrix elements for FMO and LHCII

Figures S1 and S2 show selected memory kernel matrix elements for FMO and LHCII. We note that for FMO there are 1225 unique memory kernel matrix elements and for LHCII there are 19306 unique elements.

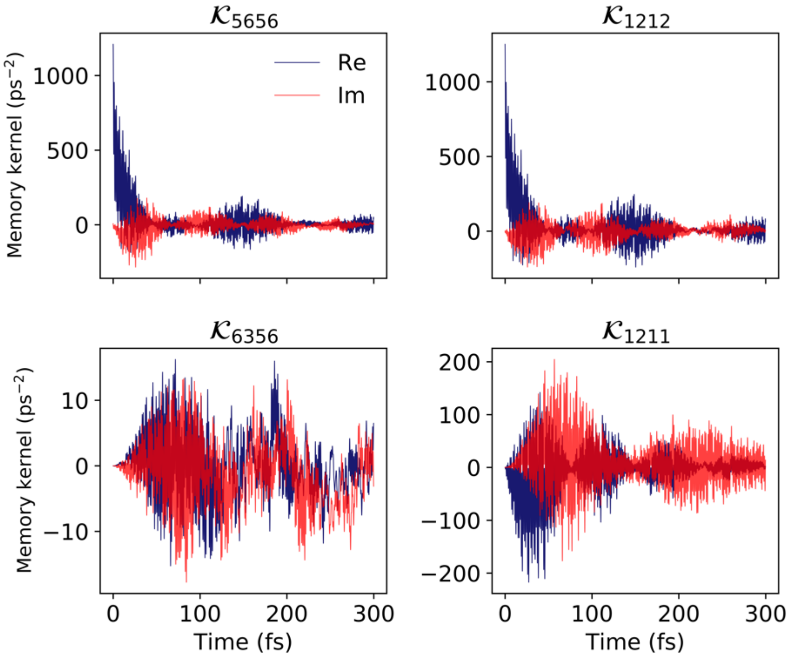


**Figure S1.** Selected memory kernel matrix elements for MF-GQME for the FMO model. The dark blue line is the real part and the red line the imaginary part. The notation with four numbers denotes the initial and final states, e.g. 6356 corresponds to $\hat{A}_m = |6\rangle\langle 3|$ and $\hat{A}_n = |5\rangle\langle 6|$.

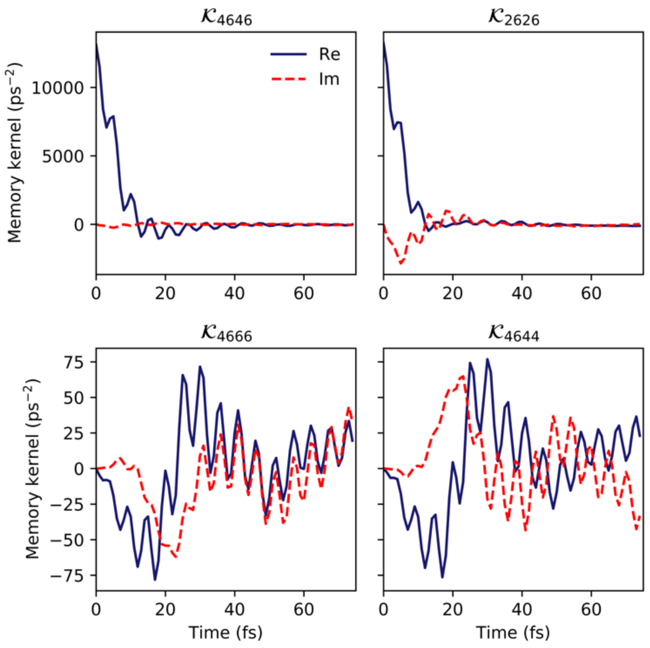


**Figure S2.** Selected memory kernel matrix elements for MF-GQME with the LHCII model. The dark blue line is the real part and the red line the imaginary part. The notation with four numbers denotes the initial and final states, e.g. 4646 corresponds to $\hat{A}_m = |4\rangle\langle 6|$ and $\hat{A}_n = |4\rangle\langle 6|$.

## 2. Performance of the selective sampling algorithm

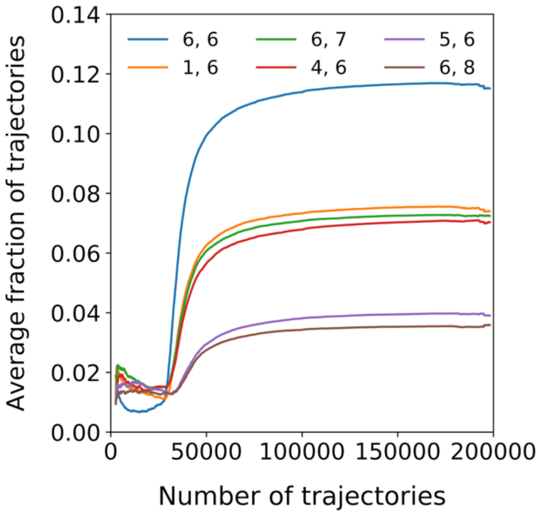


**Figure S3.** Average fraction of trajectories assigned to memory kernel level initial conditions for LHCII. The six initial conditions shown are those with the highest average weight over all 200,000 trajectories.

Figure S3 shows the weight of several initial conditions as a function of number of trajectories added. The six initial conditions with the largest average weights are shown. Figure S4 shows the mean absolute deviation as a function of trajectories for selective and uniform sampling.

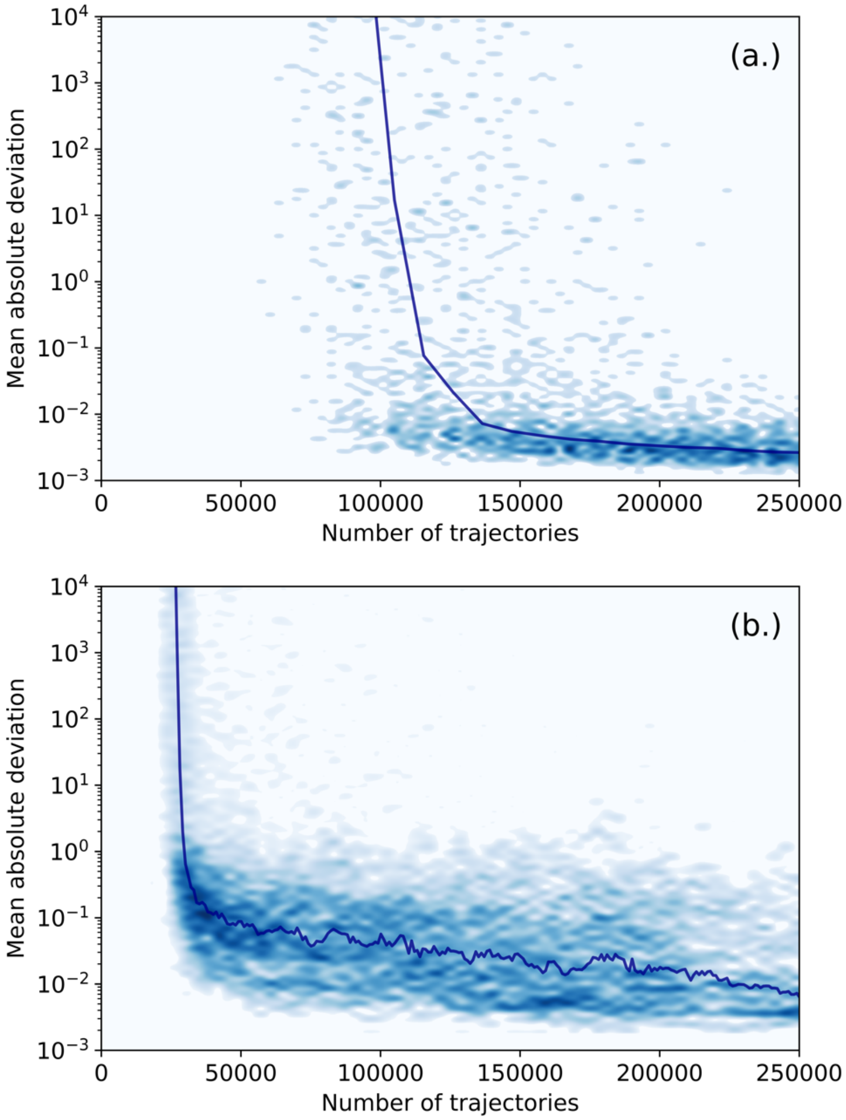


**Figure S4.** Mean absolute deviation for uniform sampling (panel a) and selective sampling (panel b) as a function of number of trajectories. The intensity of the color corresponds to the number of realizations with a given error at a given total number of trajectories, and the solid line shows the median error.
